# Supplementary material for: Universal Features of Annealing and Aging in Compaction of Granular Piles
Source: arXiv:2010.01991 source file (2020-12-15)
Supplement: Supplementary file 1 [file suplementary_material.pdf]

# Supplementary Information

In the following, we provide supplementary information to demonstrate the robustness of the results presented in the main manuscript. This is motivated by the concern that the effects of gravity might lead to significantly and qualitatively altered results throughout the granular pile. We show that the stratification merely affects quantitative variations while leaving the physical concepts that drive the observed behavior unchanged.

It needs to be appreciated that the acceleration $\Gamma$, that is by necessity uniformly applied to the entire pile, impacts different layers of the pile with a gradual variation. Although the precise meaning of this analogy is still being debated, $\Gamma$ plays the role that temperature occupies in a thermally activated systems. Thus, the observed stratification is the analogue of a gradual (monotone) variation in the effective temperature along the height of the pile. Even at the low acceleration ($\Gamma_q = 1.3$) used in our aging protocol, the bottom of the pile remains entirely frozen while a small layer on top becomes highly excited and quasi equilibrates. For illustration, we have included a brief animation (see "Movie S1") of the evolution during a *single* tap at $\Gamma_q$ that shows both, the instantaneous velocities and contact numbers of individual grains. A snapshot taken from that animation is shown in Fig. S1(a). (Note that most of the simulation time is spent in the end ensuring that the pile has become sufficiently static, as our reported measurements *only* concern the static configurations attained between taps!)

In Fig. S1(b), we show one such static configuration of the entire pile by slicing the three-dimensional, cylindrical pile right down the center axis. Red and blue coloring distinguish between the two types of mildly bi-disperse particles. The white-dashed boxes mark the three disk-shaped regions in which we have measured our observables, each containing

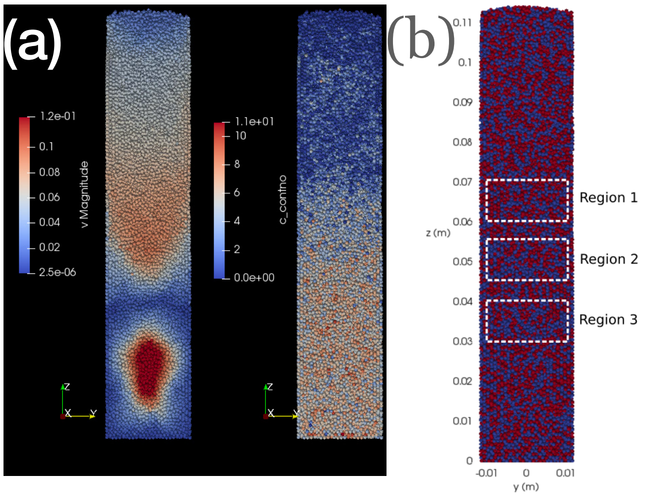


Figure S1: (a) Snapshot taken during an animation of the tap dynamics. The movie, enclosed as "Movie S1.avi" in the SI, shows for each grain within view the instantaneous speed (left) and contact number (right), according to the color-scale provided. (b) Schematic of the three regions in the pile used in the analysis. In this snapshot, red and blue refer to the two different sizes of grains used.

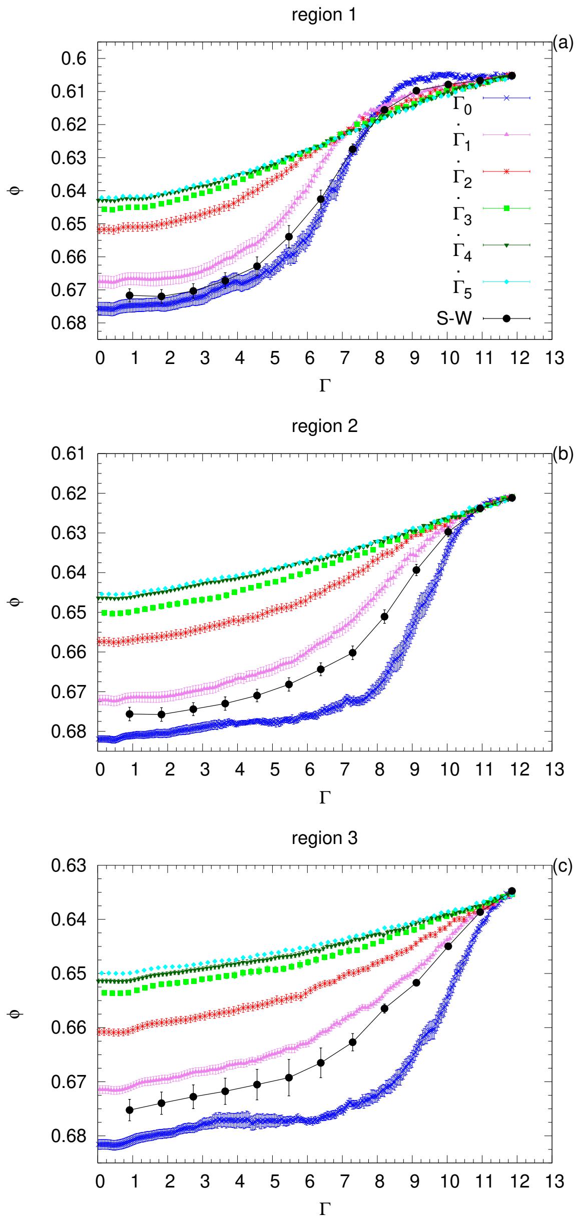


Figure S2: Average system density $\phi$ in (a) Region 1, (b) Region 2, and (c) Region 3, defined in Fig. S1(b), as a function of the dimensionless acceleration $\Gamma$ for different annealing protocols: a step-wise protocol (S-W) (150 taps in each acceleration) and a *gradually* reduced acceleration after each tap at different constant speeds, $-\dot{\Gamma}_i = v_i \times 10^{-2}$, with $v_1 = 0.279$, $v_2 = 0.808$, $v_3 = 1.373$, $v_4 = 2.334$, $v_5 = 3.83$, $v_6 = 6.747$. The results for (a-c) are obtained (and averaged over) within the same 10 independent realizations, where error bars corresponding to the standard error of the mean.

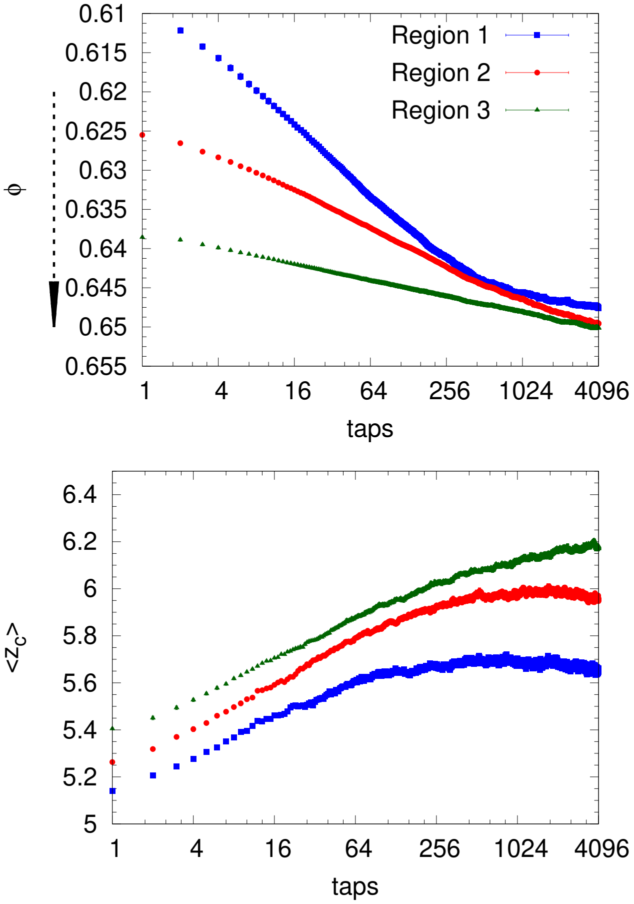


Figure S3: Average density $\phi$ within the three regions of the granular pile (top) as well as the average number of contacts, $\langle z_c \rangle$ (bottom), as a function of number of taps. The data is obtained after a quench from $\Gamma_{\text{high}} = 11$ to $\Gamma_q = 1.3$ and is averaged over 10 runs.

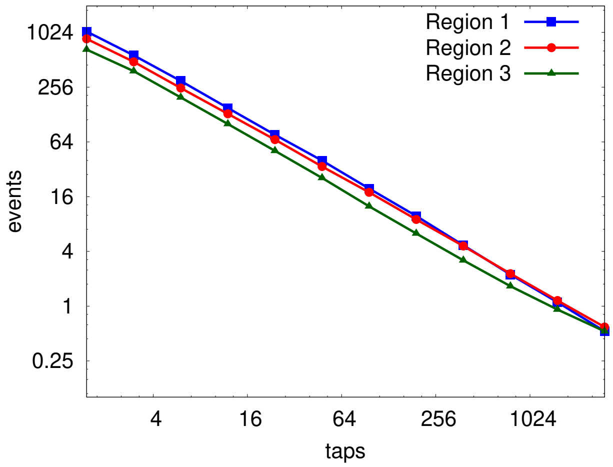


Figure S4: Number of new record events per unit time (tap), where an "event" occurs when a particle increases its coordination number from $z_c \to z_c + 1$ for the first time.

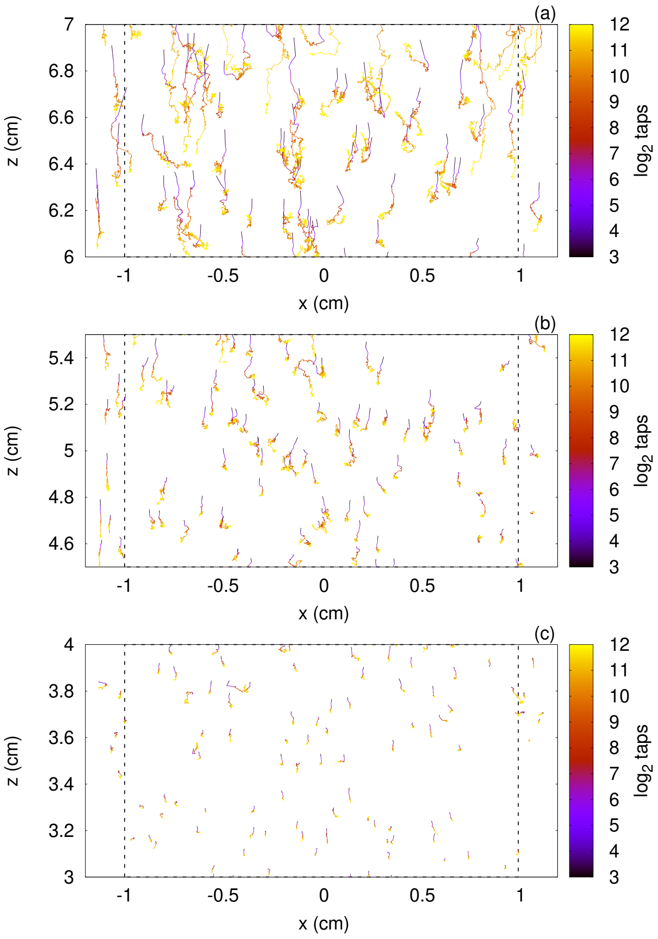


Figure S5: Tracking of displacements with time, according to the provided color code, for some randomly selected particles in regions 1, 2 and 3 in panels (a), (b), and (c), respectively.

more than 3500 particles. They are sufficiently removed from the side-walls (not shown) to avoid any crystallization effects there. Data shown in the main part of the manuscript exclusively refer to "Region 2", while we present the same data side-by-side for all three regions in the following.

In Fig. S2(a-c) we show the equivalent of Fig. 1 for the three regions. While there are quantitative differences in the attained densities at different values of $\Gamma$ for the various annealing protocols, the overall qualitative behavior remains the same in all regions. However, note that a projected glass transition, based on the value of $\Gamma$ at which each protocol falls out of equilibrium and follows a distinct evolution, would be marked differently for different regions, i.e., for different heights within the pile.

In Fig. S3 we present the equivalent of Fig. 2 in the main text that shows the average packing fraction as well as the average number of contacts as a function of the number of taps, measured over the different regions. We obtain generally logarithmic behavior for the densities, at least initially, but with different pre-factors. In the highest region (Region

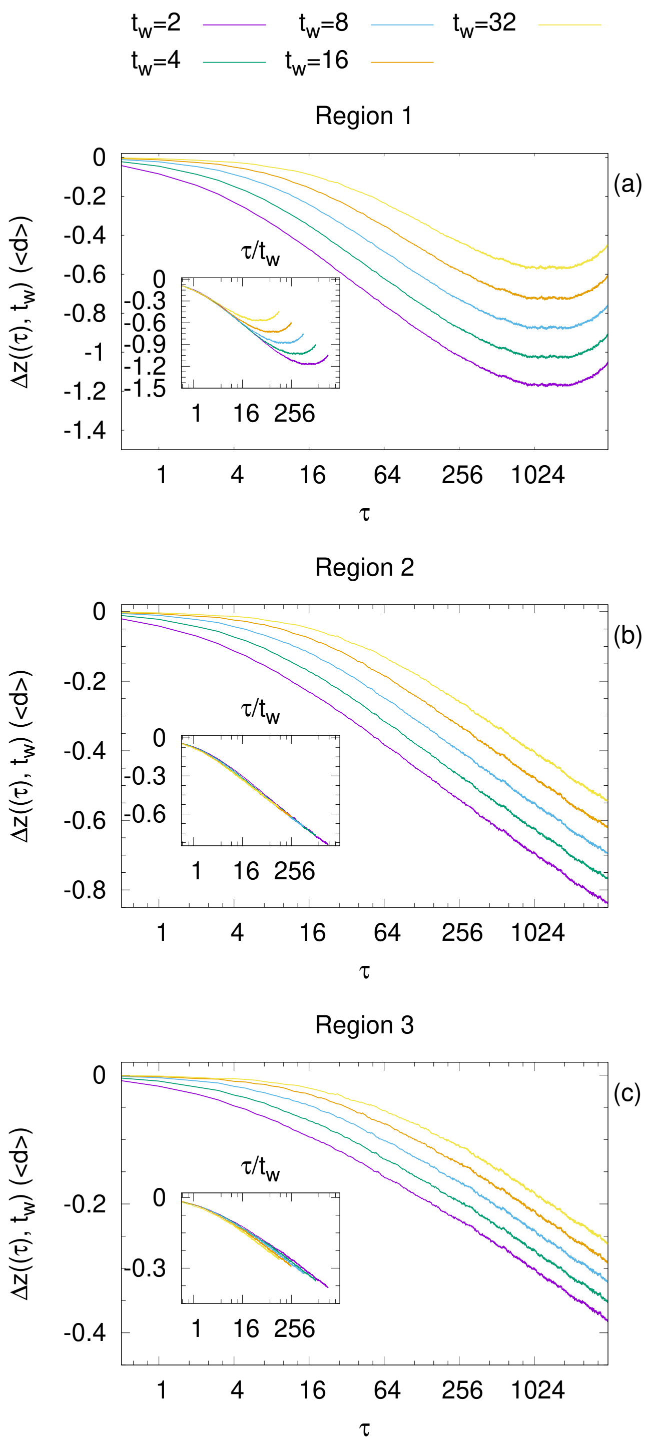


Figure S6: Plot of downward displacement averaged over all grains within each region as a function of lag-time $\tau = t - t_w$, relative to each grain's position at time $t_w$ after the quench. *Insets:* Collapse of the data in the main panel when plotted as function of $\tau/t_w$.

1), saturation effects emerge at long times, potentially indicative of some convective behavior near the wall arising due to the lower aspect ratio of this pile when compared to the Chicago experiment [1, 2]. These are more pronounced in the average contact numbers, which are somewhat correlated with density. But their average says little about the distribution and geometric arrangement of those contacts.

The nature of contacts appears to be more succinctly captured by its extremal measure, namely the records produced in achieving a larger contact number. The rate at which those records are produced remains consistently hyperbolic, as Fig. S4 shows. As to be expected, there is a slight decrease in the rate for lower regions, with a reduced activity overall.

A good illustration of the behavior for individual particles with increasing number of taps is provided in Fig. S5, which expands on Fig. 4. Although the absolute level of downward displacements changes considerably with height, the qualitative features appear to change little, as found in the previous figures. This is also reflected in the quantitative measure of the average downward displacement in Fig. S6, complementing Fig. 5. Despite the significant change in scale (see y-axis) by about a factor of two between each panel, the overall behavior remains the same. (Again, in the higher region, Region 1, some convective behavior is affecting displacements at later times.)

*Movie S1:* The enclosed Movie S1 provides an animation for the evolution of the pile during a single tap. It shows grains within a slice of the cylindrical pile, cut down along its central axis. The pile is depicted twice, showing for each grain within view the instantaneous speed (left) and contact number (right), according to the color-scale provided. (For a snapshot from the movie, see also Fig. S1.) In the movie, the pile is accelerated upward with a semi-sinusoidal wave (the "tap"), causing the grains first to launch up and then to fall back down, bounce, and settle down while dissipating their kinetic energy. Although the actual tap is brief, it takes a much longer time for all grains to have dissipated their kinetic energy sufficiently to consider the pile as being in static equilibrium again.


[1] E. Nowak, J. Knight, M. Povinelli, H. Jaeger, and S. Nagel, Powder Technology **94**, 79 (1997).

[2] E. R. Nowak, J. B. Knight, E. Ben-Naim, H. M. Jaeger, and S. R. Nagel, Phys. Rev. E **57**, 1971 (1998).
